# Supplementary material for: Multi-style Generative Network for Real-time Transfer
Source: arXiv:1703.06953 source file (2017-11-16)
Supplement: Supplementary file 1 [file appendix.tex]

\input{sections/addition}

\appendix
\section{Additional Results}

We make comparison with a concurrent work Huang {\it et al.}~\cite{huang2017arbitrary} using the same pictures of the main paper. 
Figure~\ref{fig:compare2} shows that both approaches achieve good perceptive quality, but MSG-Net handles the target styles better than the other work. Especially for transferring the textures, MSG-Net preserves both the colors and textures in the style images, while the other work  scatters mosaic-like textures to each image. 
However, this comparison is not inferring that our approach is better, but showing the differences of the applications and motivations of these two works. Huang {\it et al.} is aiming at arbitrary styles, while our proposed MSG-Net is targeting at a set of specific styles and transferring them without losing quality compared with existing approaches.

%\input{figures/all}

%Additionally, we include the example results for another 11 styles in Figure~\ref{fig:all} that are omitted form Figure~\ref{fig:9styles} of the main paper due to space constraints (20 styles in total). 
